# Supplementary material for: Towards Privacy-, Budget-, and Deadline-Aware Service Optimization for Large Medical Image Processing across Hybrid Clouds
Source: arXiv:2401.12597 source file (2024-01-23)
Supplement: Supplementary file 1 [file appendix.tex]

\section{Data}

\begin{table*}[!ht]
    \centering
    \caption{The specification of GPU cloud virtual machines.}
    \begin{tabular}{cccccccc}
     \toprule
         \textbf{Node} & \textbf{GPUs per Server} & \textbf{vCPUs} & \textbf{RAM (GB)} & \textbf{Local Storage (GB)} & \textbf{Location} & \textbf{Price (/Hour)} & \textbf{RPerf} \\ 
         \midrule
         i & Tesla T4 16GB $\times$ 1  & 4 & 7.8  & 40 & Amsterdam, Netherlands& 0 & 1/2.23 \\ 
         ii & Tesla T4 16GB $\times$ 1  & 4 & 7.8  & 40 & Amsterdam, Netherlands& 0 & 1/2.23 \\ 
         iii & RTX 3090 24GB $\times$ 1 & 48 & 125 & 40 & Valencia, Spain & 0 & 1 \\
         iv & RTX 3090 24GB $\times$ 1 & 48 & 125 & 40 & Stavanger, Norway & 0 & 1 \\
         v & A100 PCIE 80GB  & 2 & 4 & 100 & Illinois, USA & \$2.15  & 1/1.55\\ 
         vi & A100 PCIE 40GB  & 2 & 4 & 100 & Illinois, USA & \$2.01 & 1/1.55\\ 
         vii & V100 PCIE 16GB & 2 & 4 & 100 & Illinois, USA & \$0.81 & 1/1.62 \\ 
         viii & RTX A6000 48GB & 2 & 4 & 100 & New York, USA & \$1.27 & 1/0.9 \\
         ix & RTX A6000 48GB & 2 & 4 & 100 & Illinois, USA & \$1.27 & 1/0.9 \\
         x & RTX A5000 24GB & 2 & 4 & 100 & New York, USA & \$0.78 & 1/1.22 \\
         xi & RTX A5000 24GB & 2 & 4 & 100 & Illinois, USA & \$0.78 & 1/1.22 \\
         xii & RTX A5000 24GB & 2 & 4 & 100 & Nevada, USA & \$0.78 & 1/1.22 \\
         xiii & RTX A4000 16GB & 2 & 4 & 100 & New York, USA & \$0.63 & 1/1.57 \\
         xiv & RTX A4000 16GB & 2 & 4 & 100 & Illinois, USA & \$0.63 & 1/1.57 \\
         xv & A40 48GB & 2 & 4 & 100 & New York, USA & \$1.27 & 1/0.93 \\
         xvi & A40 48GB & 2 & 4 & 100 & Illinois, USA & \$1.27 & 1/0.93 \\
         xvii & A40 48GB & 2 & 4 & 100 & Nedada, USA & \$1.27 & 1/0.93 \\
         xviii & QUADRO RTX 5000 6GB & 2 & 4 & 100 & New York, USA & \$0.59 & 1/1.78 \\
         xix & QUADRO RTX 5000 6GB & 2 & 4 & 100 & Illinois, USA & \$0.59 & 1/1.78 \\
         xx & QUADRO RTX 5000 6GB & 2 & 4 & 100 & Nevada, USA & \$0.59 & 1/1.78 \\
         xxi & QUADRO RTX 4000 8GB & 2 & 4 & 100 & New York, USA & \$0.28 & 1/2.38 \\
         xxii & QUADRO RTX 4000 8GB & 2 & 4 & 100 & Illinois, USA & \$0.28 & 1/2.38 \\
         xxiii & QUADRO RTX 4000 8GB & 2 & 4 & 100 & Nevada, USA & \$0.28 & 1/2.38 \\
         xxiv & RTX 3060 TI 8GB & 4 & 12 & 80 & Norway & \$0.34 & 1/1.74 \\
         xxv & RTX 3090 24GB & 4 & 24 & 80 & Norway & \$0.59 & 1 \\
         xxvi & RTX 3090 24GB & 4 & 24 & 80 & Iceland & \$0.59 & 1 \\
         xxvii & RTX 3080 10GB & 4 & 12 & 80 & Norway & \$0.50 & 1/1.14 \\
         xxviii & RTX 3080 10GB & 4 & 12 & 80 & Iceland & \$0.50 & 1/1.14 \\
         xxix & V100 PCIE 16GB & 8 & 120 & 900 & India & \$1.07 & 1/1.62 \\
         \bottomrule
    \end{tabular}
    \label{tab: infracloud}
\end{table*}
\section{Figures}
